# Supplementary material for: SCVRL: Shuffled Contrastive Video Representation Learning
Source: arXiv:2205.11710 source file (2022-05-24)
Supplement: Supplementary file 1 [file X_supplementary.tex]

%!TEX root = ../main.tex

\appendix

% --- PDF will be split by an editor (e.g. macOS preview), so need to restart from page 1
\setcounter{page}{1}

\input{fig/Supplementary/nn_sup1}
\section{Video Retrieval Comparison}
We provide eight additional examples in Fig. \ref{fig:nn_sup1}, \ref{fig:nn_sup2}, and \ref{fig:nn_sup3} for the video retrieval comparison between our \ours{} and CVRL, as discussed in Sec. 4.3 in the main paper. For each query, we show the top three nearest-neighbor based on the representations of CVRL and SCVRL. For each video, we show the first, middle and last frame. The ground-truth class is provided on top. 
The figures illustrate that SCVRL consistently captures better motion information. CVRL retrieves videos mainly based on appearance and neglecting the temporal information inherent in the query video. This can be clearly seen in Query 1, 2, 4, and 7. CVRL confuse videos from classes, e.g., 'Moving sth. up' and 'Moving sth. down' (Query 1) in which the temporal order of the frames defines the only difference between the classes. More details to each query can be found in the corresponding caption.

\input{fig/Supplementary/nn_sup2}
\white{This is a placeholder so the figure in the next column is at the top  ----- placeholder -----placeholder -----placeholder -----placeholder -----placeholder -----placeholder -----placeholder -----placeholder -----placeholder -----placeholder -----placeholder -----placeholder -----placeholder -----placeholder -----placeholder ------- placeholder -----placeholder -----placeholder -----placeholder -----placeholder -----placeholder -----placeholder -----placeholder -----placeholder -----placeholder -----placeholder -----placeholder -----placeholder -----placeholder -----placeholder ------- placeholder -----placeholder -----placeholder -----placeholder -----placeholder}
